# Supplementary material for: Born-Oppenheimer approximation in optical cavities: from success to breakdown
Source: arXiv:2009.08304 source file (2020-09-17)
Supplement: Supplementary file 1 [file h2co_cavity_SI_arxiv.pdf]

**Supporting Information for:**

# Born–Oppenheimer approximation in optical cavities: from success to breakdown

Csaba Fábri,[1,2,a] Gábor J. Halász,[3] Lorenz S. Cederbaum,[4] and Ágnes Vibók[5,6,b]

[1] *Laboratory of Molecular Structure and Dynamics, Institute of Chemistry, Eötvös Loránd University, Pázmány Péter sétány 1/A, H-1117 Budapest, Hungary*

[2] *MTA-ELTE Complex Chemical Systems Research Group, P.O. Box 32, H-1518 Budapest 112, Hungary*

[3] *Department of Information Technology, University of Debrecen, P.O. Box 400, H-4002 Debrecen, Hungary*

[4] *Theoretische Chemie, Physikalisch-Chemisches Institut, Universität Heidelberg, Im Neuenheimer Feld 229, 69120 Heidelberg, Germany*

[5] *Department of Theoretical Physics, University of Debrecen, PO Box 400, H-4002 Debrecen, Hungary*

[6] *ELI-ALPS, ELI-HU Non-Profit Ltd, H-6720 Szeged, Dugonics tér 13, Hungary*

[a] Electronic mail: ficsaba@caesar.elte.hu

[b] Electronic mail: vibok@phys.unideb.hu

# I. THE $H_2CO$ MOLECULE AND TECHNICAL DETAILS OF THE 6D COMPUTATIONS

The planar ground-state (X) equilibrium structure of $H_2CO$ ($C_{2v}$ point-group symmetry) is shown in Fig. 1. The definition of the body-fixed Cartesian axes in Fig. 1 follows the Mulliken convention.[1] The normal modes of $H_2CO$ are summarized in Fig. 2 and Table I. In the excited electronic state (A) $H_2CO$ has two equivalent nonplanar equilibrium structures ($C_s$ point-group symmetry) that are connected by a planar transition state structure ($C_{2v}$ point-group symmetry).

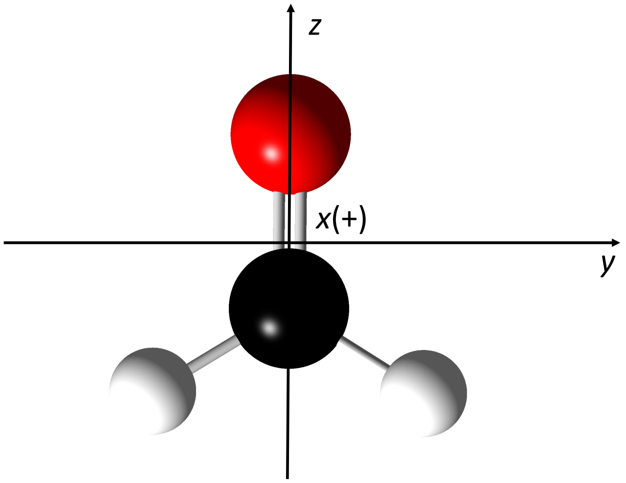


Figure 1. Equilibrium structure of the $H_2CO$ molecule in its electronic ground state (X) and definition of the body-fixed Cartesian axes (the $x$ axis is directed outwards, as indicated by the + sign).

In $H_2CO$ there is no natural conical intersection (CI) in the vicinity of the Franck–Condon region. A seam of CIs has been characterized in refs. 2–4, but it is protected by a transition barrier at low energies. $H_2CO$ has the great advantage of not having any first-order nonadiabatic coupling between the ground (X) and first singlet excited (A) electronic states around its equilibrium geometry. As a consequence, light-induced nonadiabatic phenomena can be unambiguously separated from other natural nonadiabatic effects.

The six-dimensional (6D) time-independent vibrational Schrödinger equation was solved variationally by the numerically exact and general rovibrational code GENIUSH[5–7] to obtain vibrational energy levels and eigenstates for the $V_X$ and $V_A$ potential energy surfaces

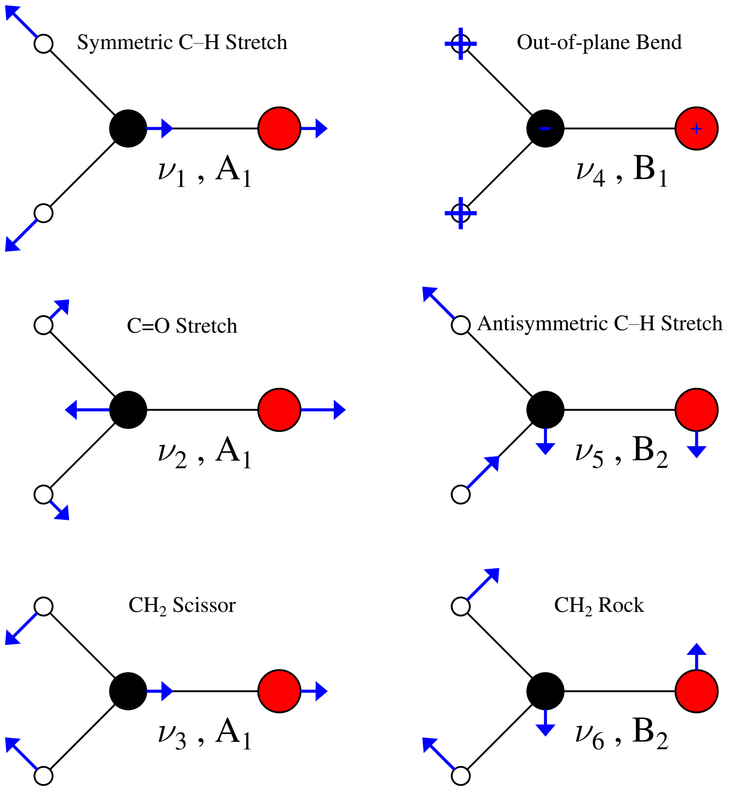


Figure 2. Normal modes of the $H_2CO$ molecule.

Table I. Normal mode labels, $C_{2v}$ irreducible representations, description of normal modes and anharmonic fundamentals (obtained by 6D variational computations in the electronic ground state (X) of $H_2CO$, in units of $cm^{-1}$).

| mode | symmetry | description | $\omega/cm^{-1}$ |
|---|---|---|---|
| $\nu_1$ | $A_1$ | sym C-H stretch | 2728.4 |
| $\nu_2$ | $A_1$ | C=O stretch | 1738.1 |
| $\nu_3$ | $A_1$ | $CH_2$ scissor | 1466.0 |
| $\nu_4$ | $B_1$ | out-of-plane bend | 1147.0 |
| $\nu_5$ | $B_2$ | antisym C-H stretch | 2819.9 |
| $\nu_6$ | $B_2$ | $CH_2$ rock | 1234.5 |

(PESs). The body-fixed Cartesian position vectors of the nuclei were parameterized using polyspherical coordinates[8] and the body-fixed axes were oriented according to the Eckart conditions[9] using the equilibrium structure of the X electronic state as reference structure. A symmetry-adapted 6D direct-product discrete variable representation (DVR) basis and

atomic mass values $m_\mathrm{C} = 12.0\,\mathrm{u}$, $m_\mathrm{O} = 15.994915\,\mathrm{u}$ and $m_\mathrm{H} = 1.007825\,\mathrm{u}$ were employed throughout the 6D vibrational eigenstate computations.

The permanent and transition dipole moment surfaces (PDM and TDM) were generated by a second-order Taylor expansion using the polyspherical coordinates defined above. The Taylor series are centered at the equilibrium structure of the X electronic state (TDM and X-state PDM) and at the planar transition state structure of the A electronic state (A-state PDM), respectively. The PDM and TDM components were referenced in the Eckart frame described above and the necessary dipole derivatives were evaluated numerically at the CAM-B3LYP/6-31G* level of theory.

## II. TECHNICAL DETAILS OF THE 2D($\nu_2$,$\nu_4$) AND 1D($\nu_4$) COMPUTATIONS

The 2D($\nu_2$,$\nu_4$) and 1D($\nu_4$) models of $H_2CO$ were defined by evaluating the normal coordinates corresponding to the planar transition state structure of the A electronic state and setting the values of the inactive normal coordinates to zero. The 2D($\nu_2$,$\nu_4$) and 1D($\nu_4$) PESs ($V_\mathrm{X}$ and $V_\mathrm{A}$) and TDM surfaces were calculated at the CAM-B3LYP/6-31G* level of theory. The energy levels and eigenstates of the coupled molecule-cavity system were computed by diagonalizing the Hamiltonian defined in Eq. (2) of the manuscript in the direct-product basis of 2D or 1D DVR basis functions and Fock states of the cavity mode with $n = 0, 1, 2, 3$.

The polaritonic (adiabatic) PESs were obtained by diagonalizing the potential energy part of the Hamiltonian defined in Eq. (2) of the manuscript. The nonadiabatic coupling between the polaritonic PESs was neglected and the time-independent Schrödinger equation was solved for each polaritonic PES separately. The TDM was transformed into the adiabatic representation and transition amplitudes were evaluated by computing the matrix elements of the adiabatic TDM surfaces between different adiabatic eigenstates.

## III. ANALYTICAL CONSIDERATIONS FOR THE 1D($\nu_4$) MODEL

We consider only the singly-excited subspace (ground electronic state dressed with one photon and excited electronic state dressed with zero photon) and diagonalize the two-

dimensional potential energy matrix

$$\mathbf{V} = \begin{bmatrix} V_{\mathrm{A}} & W_1 \\ W_1 & V_{\mathrm{X}} + \hbar\omega_{\mathrm{c}} \end{bmatrix} \tag{1}$$

with $W_1 = -g\mu$ where $g$ and $\mu$ denote the coupling strength parameter and the TDM, respectively. This yields the diagonal matrix $\mathbf{V}_{\mathrm{ad}} = \mathbf{U}^{\dagger}\mathbf{V}\mathbf{U}$ with the lower and upper polaritonic (adiabatic) PESs ($V_{-}$ and $V_{+}$) on its diagonal. The two-dimensional orthogonal matrix $\mathbf{U}$ can be parameterized with the transformation angle $\varphi$, that is,

$$\mathbf{U} = \begin{bmatrix} \cos\varphi & \sin\varphi \\ -\sin\varphi & \cos\varphi \end{bmatrix} \tag{2}$$

with

$$\varphi = \frac{1}{2}\arctan\left(\frac{2g\mu}{V_{\mathrm{A}} - V_{\mathrm{X}} - \hbar\omega_{\mathrm{c}}}\right). \tag{3}$$

As described in ref 10, the nonadiabatic coupling (NAC) between $V_{-}$ and $V_{+}$ can be obtained as the first derivative of $\varphi$ with respect to the coordinates.

Let us consider two one-dimensional harmonic PESs

$$V_{\mathrm{X}}(x) = \frac{1}{2}m\omega_{\mathrm{X}}^2 x^2 \tag{4}$$

and

$$V_{\mathrm{A}}(x) = \frac{1}{2}m\omega_{\mathrm{A}}^2 (x-d)^2 + \Delta, \tag{5}$$

where $\omega_{\mathrm{X}}$ and $\omega_{\mathrm{A}}$ refer to the harmonic frequencies of the ground and excited electronic states, $m$ is the mass, $\Delta$ is the excitation energy and $V_{\mathrm{A}}(x)$ is centered at $x = d$. The TDM is assumed to have a simple linear form,

$$\mu(x) = \mu_0 + \alpha x. \tag{6}$$

The transformation angle reads

$$\varphi(x) = \frac{1}{2}\arctan\left(\frac{2g(\mu_0 + \alpha x)}{\Delta - \hbar\omega_{\mathrm{c}} + \frac{1}{2}m\omega_{\mathrm{A}}^2(x-d)^2 - \frac{1}{2}m\omega_{\mathrm{X}}^2 x^2}\right), \tag{7}$$

which yields

$$\mathrm{NAC}(x) = \frac{mg(\mu_0 + \alpha x)\left[\omega_{\mathrm{X}}^2 x - \omega_{\mathrm{A}}^2(x-d)\right] + g\alpha\left[\Delta - \hbar\omega_{\mathrm{c}} + \frac{1}{2}m\omega_{\mathrm{A}}^2(x-d)^2 - \frac{1}{2}m\omega_{\mathrm{X}}^2 x^2\right]}{\left[\Delta - \hbar\omega_{\mathrm{c}} + \frac{1}{2}m\omega_{\mathrm{A}}^2(x-d)^2 - \frac{1}{2}m\omega_{\mathrm{X}}^2 x^2\right]^2 + 4g^2(\mu_0 + \alpha x)^2} \tag{8}$$

for the NAC.

Next, we discuss the model used in ref. 11 (called anthracene-like model therein) where the following assumptions seem to have been made:

$$\begin{aligned} \omega_{\mathrm{X}} &= \omega_{\mathrm{A}} = \omega \\ \Delta &= \hbar\omega_{\mathrm{c}} \\ \mu(x) &= \mu_0 \quad (\alpha = 0). \end{aligned} \tag{9}$$

Substituting these equations into Eq. (8) results in

$$\mathrm{NAC}(x) = \frac{4g\mu_0 m\omega^2 d}{m^2\omega^4(d^2 - 2xd)^2 + 16g^2\mu_0^2} \tag{10}$$

which becomes proportional to $g^{-1}$ for sufficiently large $g$ values at every possible value of $x$.

Finally, we investigate a model with

$$\begin{aligned} \omega_{\mathrm{X}} &> \omega_{\mathrm{A}} \\ \Delta &> \hbar\omega_{\mathrm{c}} \\ d &= 0 \\ \mu(x) &= \alpha x \quad (\mu_0 = 0), \end{aligned} \tag{11}$$

which is obviously related to the 1D($\nu_4$) model of $H_2CO$ (only the out-of-plane mode is active), although the one-dimensional PES along the $\nu_4$ normal mode has an anharmonic double-well structure in the excited electronic state of $H_2CO$. In this case the general NAC formula in Eq. (8) simplifies to

$$\mathrm{NAC}(x) = \frac{4g\alpha(\Delta - \hbar\omega_{\mathrm{c}}) - 2g\alpha m(\omega_{\mathrm{A}}^2 - \omega_{\mathrm{X}}^2)x^2}{\left[2(\Delta - \hbar\omega_{\mathrm{c}}) + m(\omega_{\mathrm{A}}^2 - \omega_{\mathrm{X}}^2)x^2\right]^2 + 16g^2\alpha^2x^2}. \tag{12}$$

It is easy to see that in this case the two diabatic PESs $V_{\mathrm{X}}(x) + \hbar\omega_c$ and $V_{\mathrm{A}}(x)$ cross at

$$x_0 = \pm\sqrt{\frac{2(\Delta - \hbar\omega_{\mathrm{c}})}{m(\omega_{\mathrm{X}}^2 - \omega_{\mathrm{A}}^2)}}, \tag{13}$$

where the NAC evaluates to

$$\mathrm{NAC}(x_0) = \frac{m(\omega_{\mathrm{X}}^2 - \omega_{\mathrm{A}}^2)}{4g\alpha}. \tag{14}$$

Both Eq. (12) and Eq. (14) suggest that the NAC is inversely proportional to $g$, implying that the NAC becomes negligible for sufficiently large $g$ values. However, evaluating NAC($x$) of Eq. (12) at $x = 0$ results in

$$\mathrm{NAC}(0) = \frac{g\alpha}{\Delta - \hbar\omega_\mathrm{c}}, \tag{15}$$

which clearly shows that the NAC is proportional to $g$ at $x = 0$. This striking behaviour of the NAC indicates that the Born–Oppenheimer approximation can break down even for large $g$ values in one dimension. Finally, it is worth noting that as $\mu(0) = 0$, the gap between the two adiabatic PESs at $x = 0$ is determined solely by $\omega_c$ (and not by $g$).

## IV. ANALYTICAL CONSIDERATIONS FOR THE 2D($\nu_2$,$\nu_4$) MODEL

Next, a two-dimensional model is introduced by defining the ground-state and excited-state PESs as

$$V_\mathrm{X}(x,y) = \frac{1}{2}m\omega_{\mathrm{X1}}^2 x^2 + \frac{1}{2}m\omega_{\mathrm{X2}}^2 y^2 \tag{16}$$

and

$$V_\mathrm{A}(x,y) = \frac{1}{2}m\omega_{\mathrm{A1}}^2 x^2 + \frac{1}{2}m\omega_{\mathrm{A2}}^2 (y-d)^2 + \Delta, \tag{17}$$

and by choosing a simple linear TDM

$$\mu(x,y) = \alpha x, \tag{18}$$

depending only on $x$. This two-dimensional model is inspired by the 2D($\nu_2$,$\nu_4$) $H_2CO$ model ($x$ and $y$ would become $Q_4$ and $Q_2$, respectively, with $m = 1$ for the 2D($\nu_2$,$\nu_4$) model), although there are clearly some approximations, such as treating both PESs as a sum of two one-dimensional harmonic oscillator PESs. The form of $\mu(x,y)$ is justified by the fact that no TDM is produced for any displacement along $Q_2$ if $Q_4$ is set to zero.

Similarly to the one-dimensional model, we first evaluate the transformation angle

$$\varphi(x,y) = \frac{1}{2}\arctan\left(\frac{4g\alpha x}{2(\Delta - \hbar\omega_\mathrm{c}) + m(\omega_{\mathrm{A1}}^2 - \omega_{\mathrm{X1}}^2)x^2 + m\omega_{\mathrm{A2}}^2(y-d)^2 - m\omega_{\mathrm{X2}}^2 y^2}\right) \tag{19}$$

and then calculate the first partial derivatives of $\varphi(x,y)$ with respect to $x$ and $y$. It is easy to see that a LICI arises at $(x_0, y_0)$ in the two-dimensional case if

$$x_0 = 0 \tag{20}$$

(zero coupling) and

$$\frac{1}{2}m\omega_{\mathrm{X2}}^2 y_0^2 = \frac{1}{2}m\omega_{\mathrm{A2}}^2 (y_0 - d)^2 + \Delta - \hbar\omega_{\mathrm{c}} \tag{21}$$

(degeneracy of the two diabatic PESs).

As the general formulae for $\frac{\partial\varphi(x,y)}{\partial x}$ and $\frac{\partial\varphi(x,y)}{\partial y}$ are rather complicated, we limit the discussion to the $x = x_0 = 0$ special case (this is a necessary condition for the LICI) and obtain

$$\mathrm{NAC}_x(0,y) = \frac{\partial\varphi(x,y)}{\partial x}\bigg|_{x=0} = \frac{2g\alpha}{2(\Delta - \hbar\omega_{\mathrm{c}}) + m\omega_{\mathrm{A2}}^2(y-d)^2 - m\omega_{\mathrm{X2}}^2 y^2} \tag{22}$$

and

$$\mathrm{NAC}_y(0,y) = \frac{\partial\varphi(x,y)}{\partial y}\bigg|_{x=0} = 0. \tag{23}$$

If the condition in Eq. (21) is fulfilled, $\mathrm{NAC}_x$ of Eq. (22) becomes singular, as it should be the case at the LICI.

## REFERENCES


[1]R. S. Mulliken, J. Chem. Phys. **23**, 1997 (1955).

[2]M. Araujo, B. Lasorne, M. J. Bearpark, and M. A. Robb, J. Phys. Chem. A **112**, 7489 (2008).

[3]M. Araújo, B. Lasorne, A. L. Magalhães, G. A. Worth, M. J. Bearpark, and M. A. Robb, J. Chem. Phys. **131**, 144301 (2009).

[4]M. Araújo, B. Lasorne, A. L. Magalhães, M. J. Bearpark, and M. A. Robb, J. Phys. Chem. A **114**, 12016 (2010).

[5]E. Mátyus, G. Czakó, and A. G. Császár, J. Chem. Phys. **130**, 134112 (2009).

[6]C. Fábri, E. Mátyus, and A. G. Császár, J. Chem. Phys. **134**, 074105 (2011).

[7]A. G. Császár, C. Fábri, T. Szidarovszky, E. Mátyus, T. Furtenbacher, and G. Czakó, Phys. Chem. Chem. Phys. **14**, 1085 (2012).

[8]X. Chapuisat and C. Iung, Phys. Rev. A **45**, 6217 (1992).

[9]C. Eckart, Phys. Rev. **47**, 552 (1935).

[10]G. J. Halász, Á. Vibók, M. Šindelka, N. Moiseyev, and L. S. Cederbaum, J. Phys. B: At. Mol. Opt. Phys. **44**, 175102 (2011).

[11]J. Galego, F. J. Garcia-Vidal, and J. Feist, Phys. Rev. X **5**, 041022 (2015).
